# Supplementary material for: Generalized Contrastive Learning for Multi-Modal Retrieval and Ranking
Source: arXiv:2404.08535 source file (2025-04-27)
Supplement: Supplementary file 1 [file appendix.tex]

\setcounter{section}{0}

\setcounter{table}{0}

\setcounter{figure}{0}

\input{table_dataset_ comparisons}
